# Supplementary material for: System Characterization of Dispersive Readout in Superconducting Qubits
Source: arXiv:2402.00413 source file (2024-02-01)
Supplement: Supplementary file 1 [file appendix.tex]

The output wave $B$ is amplified and mixed to an intermediate frequency (IF) between 10 MHz and 250 MHz with an IQ mixer.
The IF I and Q mixer outputs are filtered and sample in a pair of analogy to digital converters (ADC).
The I and Q signals coming from the mixer are
\begin{align*}
  I(t) =& \Re \left[ B(t)\exp \left( i (\omegaframe - \Omega) t \right) \right] \\
  Q(t) =& \Im \left[ B(t)\exp \left( i (\omegaframe - \Omega) t \right) \right]
\end{align*}
where $\Omega$ is the mixer's local oscillator frequency.
Defining $Z(t) = I(t) + i Q(t)$, we then digitally compute the sum
\begin{align*}
  Z
  =& \sum_{n=1}^N Z(t_n) \exp(-i (\omegaframe - \Omega) t_n) w(t_n) \\
  =& \sum_{n=1}^N B(t_n) w(t_n)
\end{align*}
arriving at a single complex number $Z$ which is interpreted as a point in the IQ plane.
Here $t_n = n \delta t$ is the $n^{\text{th}}$ sample time, $\delta t = 1 \, \text{ns}$ is the ADC sampling interval, $N = t / \delta t$ is the number of samples corresponding to a total measurement time of $t$, and $w$ is a weight function chosen to optimize the SNR.
